# Supplementary material for: Online False Discovery Rate Control for LORD & SAFFRON Under Positive, Local Dependence
Source: arXiv:2110.08161 ancillary file (2022-02-10)
Supplement: Supplementary file 1 [file saffron-fdr-pos-dependence-v8_no-tau-notation_supp.pdf]

# Supplementary Materials for *SAFFRON and LORD Ensure Online Control of the False Discovery Rate Under Positive Dependence*

Aaron Fisher\*

October 26, 2021

## Contents

|                                                                              |          |
|------------------------------------------------------------------------------|----------|
| <b>A Proof of Theorem 2</b>                                                  | <b>1</b> |
| A.1 Proof of Lemma A.1 . . . . .                                             | 2        |
| A.2 Applying Lemma A.1 to prove Theorem 2 . . . . .                          | 2        |
| <b>B Simplified implementations of LORD &amp; SAFFRON</b>                    | <b>4</b> |
| B.1 SAFFRON & LORD algorithms . . . . .                                      | 4        |
| B.2 Eqs (5) and (6) as special cases of LORD and SAFFRON . . . . .           | 4        |
| B.3 Monotonicity of proposed algorithms . . . . .                            | 6        |
| B.3.1 LORD with dynamic spending proportions and planning ahead . . . . .    | 7        |
| B.3.2 SAFFRON with dynamic spending proportions and planning ahead . . . . . | 8        |

## Brief note on cross-references

Throughout this supplement, we use letter prefixes when referring to items within the supplementary materials (e.g., Lemma A.1 in Section A of the supplement), and use regular numeric references for items in the main text (e.g., Theorem 2 in Section 3.1 of the main text).

## A Proof of Theorem 2

We start by showing FDR control under a weaker condition that is implied by Conditions 1 & 2. Roughly speaking, this new condition says that lower p-values in the early stages of testing are generally associated with a larger total number of rejections by the later stages of testing.

*Condition A.1.* (Stronger signal implies more discoveries) For any  $u \in [0, 1]$  and any  $i, t \in \mathbb{N}$  satisfying  $i \leq t$  and  $i \in \mathcal{H}_0$ , we have

$$\text{Cov} \left( \frac{1}{|\mathcal{R}_t| \vee 1}, \mathbf{1}(P_i \leq u) \mid \mathcal{F}_{i-1} \right) \leq 0.$$

In the next lemma, we use Condition A.1 to show FDR control.

**Lemma A.1.** *Suppose that, for each stage  $t$ , the set of variables  $\mathcal{F}_{t-1}$  is a deterministic function of the previous p-values  $(P_1, \dots, P_{t-1})$ , and that  $\alpha_t$  and  $\lambda_t$  are deterministic functions of  $\mathcal{F}_{t-1}$ . Suppose also that, for all  $i \in \mathcal{H}_0$  and all  $u \in [0, 1]$ , we have  $\mathbb{P}(P_i \leq u \mid \mathcal{F}_{i-1}) \leq u$ . The following two results hold.*

1. *Under Condition A.1, any method of selecting thresholds  $\{\alpha_i\}_{i \in \mathbb{N}}$  such that  $\widehat{\text{FDR}}_0(t) \leq \alpha$  for all  $t \in \mathbb{N}$  (e.g., LORD) ensures that  $\text{FDR}(t) \leq \alpha$ .*

---

\*Foundation Medicine Inc.; 150 Second St, Cambridge, MA 02141

2. Under Condition A.1, any method of selecting parameters  $\{\alpha_i, \lambda_i\}_{i \in \mathbb{N}}$  such that  $\widehat{FDR}_\lambda(t) \leq \alpha$  for all  $t \in \mathbb{N}$  (e.g., SAFFRON) ensures that  $FDR(t) \leq \alpha$ .

We prove Lemma A.1 in Section A.1, and then use it to show Theorem 2 in Section A.2.

### A.1 Proof of Lemma A.1

*Proof.* We start by building on Condition A.1, which states that indicators of low p-values are negatively correlated with  $(|\mathcal{R}_t| \vee 1)^{-1}$ . It follows from Condition A.1 that indicators of *high* p-values are *positively* correlated with  $(|\mathcal{R}_t| \vee 1)^{-1}$ . That is, for any  $u \in [0, 1]$  and any  $i, t \in \mathbb{N}$  satisfying  $i \leq t$  and  $i \in \mathcal{H}_0$ , we have

$$\begin{aligned} \text{Cov} \left( \frac{1}{|\mathcal{R}_t| \vee 1}, \mathbf{1}(P_i > u) \mid \mathcal{F}_{i-1} \right) &= \text{Cov} \left( \frac{1}{|\mathcal{R}_t| \vee 1}, 1 - \mathbf{1}(P_i \leq u) \mid \mathcal{F}_{i-1} \right) \\ &= -\text{Cov} \left( \frac{1}{|\mathcal{R}_t| \vee 1}, \mathbf{1}(P_i \leq u) \mid \mathcal{F}_{i-1} \right) \\ &\geq 0. \end{aligned} \tag{A.1}$$

Next, we break down the  $FDR(t)$  metric into a summation over the null indices.

$$\begin{aligned} FDR(t) &= \mathbb{E} \left[ \frac{\sum_{\{i \in \mathcal{H}_0: i \leq t\}} \mathbf{1}(P_i \leq \alpha_i)}{|\mathcal{R}_t| \vee 1} \right] \\ &= \sum_{\{i \in \mathcal{H}_0: i \leq t\}} \mathbb{E}_{\mathcal{F}_{i-1}} \left[ \mathbb{E} \left( \frac{1}{|\mathcal{R}_t| \vee 1} \times \mathbf{1}(P_i \leq \alpha_i) \mid \mathcal{F}_{i-1} \right) \right] \\ &\leq \sum_{\{i \in \mathcal{H}_0: i \leq t\}} \mathbb{E}_{\mathcal{F}_{i-1}} \left[ \mathbb{E} \left( \frac{1}{|\mathcal{R}_t| \vee 1} \mid \mathcal{F}_{i-1} \right) \mathbb{E}(\mathbf{1}(P_i \leq \alpha_i) \mid \mathcal{F}_{i-1}) \right] && \text{by Condition A.1} \\ &\leq \sum_{\{i \in \mathcal{H}_0: i \leq t\}} \mathbb{E}_{\mathcal{F}_{i-1}} \left[ \mathbb{E} \left( \frac{1}{|\mathcal{R}_t| \vee 1} \mid \mathcal{F}_{i-1} \right) \alpha_i \right] && \text{by super-uniformity} \\ &= \sum_{\{i \in \mathcal{H}_0: i \leq t\}} \mathbb{E}_{\mathcal{F}_{i-1}} \left[ \mathbb{E} \left( \frac{\alpha_i}{|\mathcal{R}_t| \vee 1} \mid \mathcal{F}_{i-1} \right) \right]. \end{aligned} \tag{A.2}$$

For Part 1, this completes the proof, as Line (A.2) is equal to  $\mathbb{E} \left( \frac{\sum_{\{i \in \mathcal{H}_0: i \leq t\}} \alpha_i}{|\mathcal{R}_t| \vee 1} \right) \leq \mathbb{E} \left( \frac{\sum_{i \leq t} \alpha_i}{|\mathcal{R}_t| \vee 1} \right) = \widehat{FDR}_0(t) \leq \alpha$ .

For Part 2, we continue by multiplying the inner expectation in Line (A.2) by  $\frac{\mathbb{E}[\mathbf{1}(P_t > \lambda_i) \mid \mathcal{F}_{i-1}]}{1 - \lambda_i} \geq 1$ .

$$\begin{aligned} FDR(t) &\leq \sum_{\{i \in \mathcal{H}_0: i \leq t\}} \mathbb{E}_{\mathcal{F}_{i-1}} \left[ \mathbb{E} \left( \frac{\alpha_i}{|\mathcal{R}_t| \vee 1} \mid \mathcal{F}_{i-1} \right) \frac{\mathbb{E}[\mathbf{1}(P_t > \lambda_i) \mid \mathcal{F}_{i-1}]}{(1 - \lambda_i)} \right] \\ &\leq \sum_{\{i \in \mathcal{H}_0: i \leq t\}} \mathbb{E}_{\mathcal{F}_{i-1}} \left[ \mathbb{E} \left( \frac{\alpha_i \frac{\mathbf{1}(P_t > \lambda_i)}{1 - \lambda_i}}{|\mathcal{R}_t| \vee 1} \mid \mathcal{F}_{i-1} \right) \right] && \text{by Eq A.1} \\ &= \mathbb{E} \left[ \frac{\sum_{\{i \in \mathcal{H}_0: i \leq t\}} \alpha_i \frac{\mathbf{1}(P_t > \lambda_i)}{1 - \lambda_i}}{|\mathcal{R}_t| \vee 1} \right]. \end{aligned}$$

The term in expectations is upper bounded by  $\widehat{FDR}_\lambda(t)$ , and so monotonicity of expectations shows Part 2.  $\square$

### A.2 Applying Lemma A.1 to prove Theorem 2

*Proof.* All that remains is to show that Conditions 1 & 2 imply Condition A.1.

Let  $D_{r,t} \in [0, 1]^t$  be the set of possible p-values for the first  $t$  hypotheses that produce no more than  $r \vee 1$  rejections. From Condition 1, we know that  $D_{r,t}$  is an increasing set. Following steps analogous to those used

by Blanchard and Roquain (2008; see their Proposition 3.6), we can now show that, for any  $i \leq t$  satisfying  $i \in \mathcal{H}_0$ , the distribution of  $|\mathcal{R}_t| \vee 1$  given  $P_i \leq u$  and  $\alpha_i$  is stochastically decreasing in  $u$ . That is, for any  $r, t \geq 0$ , and any  $i \leq t$  satisfying  $i \in \mathcal{H}_0$ , the probability

$$\mathbb{P}(|\mathcal{R}_t| \vee 1 \leq r \mid P_i \leq u, \mathcal{F}_{i-1})$$

is nondecreasing in  $u$ .

For any  $u < u'$ , let  $\gamma = \mathbb{P}(P_i \leq u \mid P_i \leq u', \mathcal{F}_{i-1})$ . Then

$$\begin{aligned} & \mathbb{P}(|\mathcal{R}_t| \vee 1 \leq r \mid P_i \leq u', \mathcal{F}_{i-1}) \\ &= \mathbb{P}((P_1, \dots, P_t) \in D_{r,t} \mid P_i \leq u', \mathcal{F}_{i-1}) \\ &= \mathbb{E}[\mathbb{P}\{(P_1, \dots, P_t) \in D_{r,t} \mid P_i, \mathcal{F}_{i-1}\} \mid P_i \leq u', \mathcal{F}_{i-1}] \\ &= \mathbb{E}[\mathbb{P}\{(P_1, \dots, P_t) \in D_{r,t} \mid P_i, \mathcal{F}_{i-1}\} \mid P_i \leq u, \mathcal{F}_{i-1}] \gamma \\ &\quad + \mathbb{E}[\mathbb{P}\{(P_1, \dots, P_t) \in D_{r,t} \mid P_i, \mathcal{F}_{i-1}\} \mid u < P_i \leq u', \mathcal{F}_{i-1}] (1 - \gamma) \end{aligned} \tag{A.3}$$

$$\begin{aligned} & \geq \mathbb{E}[\mathbb{P}\{(P_1, \dots, P_t) \in D_{r,t} \mid P_i, \mathcal{F}_{i-1}\} \mid P_i \leq u, \mathcal{F}_{i-1}] \gamma \\ &\quad + \mathbb{E}[\mathbb{P}\{(P_1, \dots, P_t) \in D_{r,t} \mid P_i, \mathcal{F}_{i-1}\} \mid P_i \leq u, \mathcal{F}_{i-1}] (1 - \gamma) \end{aligned} \tag{A.4}$$

$$\begin{aligned} &= \mathbb{E}[\mathbb{P}\{(P_1, \dots, P_t) \in D_{r,t} \mid P_i, \mathcal{F}_{i-1}\} \mid P_i \leq u, \mathcal{F}_{i-1}] \\ &= \mathbb{P}((P_1, \dots, P_t) \in D_{r,t} \mid P_i \leq u, \mathcal{F}_{i-1}) \\ &= \mathbb{P}(|\mathcal{R}_t| \vee 1 \leq r \mid P_i \leq u, \mathcal{F}_{i-1}). \end{aligned} \tag{A.5}$$

Above, we transform Line (A.3) to Line (A.4) by applying Condition 2 to the inner probability within each line.

It follows that the distribution of  $(|\mathcal{R}_t| \vee 1)^{-1}$  given  $P_i \leq u$  and  $\mathcal{F}_{i-1}$  is stochastically *increasing* in  $u$ . To see this, from Eq (A.5) we have

$$\begin{aligned} & \mathbb{P}(|\mathcal{R}_t| \vee 1 \leq r \mid P_i \leq u, \mathcal{F}_{i-1}) \leq \mathbb{P}(|\mathcal{R}_t| \vee 1 \leq r \mid P_i \leq u', \mathcal{F}_{i-1}) \\ & \mathbb{P}(|\mathcal{R}_t| \vee 1 < r + 1 \mid P_i \leq u, \mathcal{F}_{i-1}) \leq \mathbb{P}(|\mathcal{R}_t| \vee 1 < r + 1 \mid P_i \leq u', \mathcal{F}_{i-1}) \\ & \mathbb{P}\left(\frac{1}{r+1} < \frac{1}{|\mathcal{R}_t| \vee 1} \mid P_i \leq u, \mathcal{F}_{i-1}\right) \leq \mathbb{P}\left(\frac{1}{r+1} < \frac{1}{|\mathcal{R}_t| \vee 1} \mid P_i \leq u', \mathcal{F}_{i-1}\right). \end{aligned} \tag{A.6}$$

In general, if  $P(X > a) \leq P(Y > a)$  holds for two random variables  $X, Y$  at all points  $a$  in their domain (i.e.,  $Y$  is stochastically larger than  $X$ ), then  $\mathbb{E}(X) \leq \mathbb{E}(Y)$  (see, for example, Wolfstetter et al. 1993). Thus, Eq (A.6) implies that

$$\mathbb{E}\left(\frac{1}{|\mathcal{R}_t| \vee 1} \mid P_i \leq u, \mathcal{F}_{i-1}\right) \leq \mathbb{E}\left(\frac{1}{|\mathcal{R}_t| \vee 1} \mid P_i \leq u', \mathcal{F}_{i-1}\right). \tag{A.7}$$

Applying this, we have

$$\begin{aligned} \mathbb{E}\left(\frac{\mathbf{1}(P_i \leq u)}{|\mathcal{R}_t| \vee 1} \mid \mathcal{F}_{i-1}\right) &= \mathbb{E}\left(\frac{1}{|\mathcal{R}_t| \vee 1} \mid P_i \leq u, \mathcal{F}_{i-1}\right) \mathbb{P}(P_i \leq u \mid \mathcal{F}_{i-1}) \\ &= \mathbb{E}\left(\frac{1}{|\mathcal{R}_t| \vee 1} \mid P_i \leq u, \mathcal{F}_{i-1}\right) \mathbb{E}(\mathbf{1}(P_i \leq u) \mid \mathcal{F}_{i-1}) \\ &\leq \mathbb{E}\left(\frac{1}{|\mathcal{R}_t| \vee 1} \mid \mathcal{F}_{i-1}\right) \mathbb{E}(\mathbf{1}(P_i \leq u) \mid \mathcal{F}_{i-1}). \end{aligned} \tag{A.8}$$

Where the last inequality comes from Eq (A.7), with  $u'$  set equal to 1. Eq (A.8) can be equivalently written as saying that

$$\text{Cov}\left(\frac{1}{|\mathcal{R}_t| \vee 1}, \mathbf{1}(P_i \leq u) \mid \mathcal{F}_{i-1}\right) \leq 0.$$

From here, Lemma A.1 proves the result.  $\square$

## B Simplified implementations of LORD & SAFFRON

In this section we review the full details of the LORD & SAFFRON algorithms. We then show that the simplifications in Eqs (5) & (6) are special cases of the LORD & SAFFRON algorithms, respectively. Finally, we show that all of the modified implementations described in Section 4 produce thresholds that are nonincreasing in the previous p-values.

### B.1 SAFFRON & LORD algorithms

Ramdas et al. (2018) describe a p-value  $P_i$  as being a “candidate” for rejection if  $P_i \leq \lambda_i$ . Under the condition that all stages use the same, user-specified value for  $\lambda_i$ , the authors define the SAFFRON algorithm as requiring tuning parameters  $\lambda \in (0, 1)$ ;  $W_0 \leq (1 - \lambda)\alpha$ ; and  $\{\gamma_j\}_{j=1}^\infty$  such that  $\sum_{j=1}^\infty \gamma_j = 1$ . Let  $r_j$  be the time of the  $j^{\text{th}}$  rejection, and let

$$C_{j+}(t) = \begin{cases} \sum_{i=r_j+1}^{t-1} \mathbf{1}(P_i \leq \lambda) & \text{if } r_j + 1 \leq t - 1 \\ 0 & \text{otherwise} \end{cases}$$

be the number of candidate p-values occurring between the  $j^{\text{th}}$  rejection and the  $t^{\text{th}}$  stage. Similarly, we define

$$N_{j+}(t) = \begin{cases} \sum_{i=r_j+1}^{t-1} \mathbf{1}(P_i > \lambda) & \text{if } r_j + 1 \leq t - 1 \\ 0 & \text{otherwise} \end{cases}$$

to be the number of “non-candidates” between the  $j^{\text{th}}$  rejection and the  $t^{\text{th}}$  stage. It follows that  $N_{j+}(t) = t - 1 - r_j - C_{j+}(t)$ .

SAFFRON defines  $\alpha_t = \min\{\tilde{\alpha}_t, \lambda\}$ , where  $\tilde{\alpha}_1 = W_0\gamma_1$  and

$$\begin{aligned} \tilde{\alpha}_t &= W_0\gamma_{t-C_{0+}(t)} + ((1 - \lambda)\alpha - W_0)\gamma_{t-r_1-C_{1+}(t)} + \sum_{j=2}^{|\mathcal{R}_{t-1}|} (1 - \lambda)\alpha\gamma_{t-r_j-C_{j+}(t)} \\ &= W_0\gamma_{1+N_{0+}(t)} + ((1 - \lambda)\alpha - W_0)\gamma_{1+N_{1+}(t)} + \sum_{j=2}^{|\mathcal{R}_{t-1}|} (1 - \lambda)\alpha\gamma_{1+N_{j+}(t)}, \end{aligned} \quad (\text{B.1})$$

where the summation is omitted if  $|\mathcal{R}_{t-1}| < 2$ .

The LORD algorithm described in Eq (5) of Ramdas et al. (2017) uses thresholds equivalent to  $\tilde{\alpha}_t$  (omitting the min operator), with  $\lambda$  set equal to zero.

### B.2 Eqs (5) and (6) as special cases of LORD and SAFFRON

Next, we show a relationship between Eq (6) and Eq (B.1).

*Remark B.1.* If  $W_0 = \alpha(1 - \lambda)$  and  $\gamma_i = \pi(1 - \pi)^{i-1}$  for all  $i \in \mathbb{N}$ , then  $\tilde{\alpha}_i = \bar{\alpha}_i$  for all  $i \in \mathbb{N}$ .

Remark B.1 immediately implies that Eq (6) is a special case of the SAFFRON algorithm. The LORD algorithm is nearly equivalent to the SAFFRON algorithm with  $\lambda = 0$ , with the exception that we allow  $\alpha_i > \lambda$ . In other words, if  $\lambda = 0$ , then  $\bar{\alpha}_t$  is equivalent to the threshold used by LORD in stage  $t$ . Thus, Remark B.1 also implies that setting  $W_0 = \alpha$ ,  $\lambda = 0$  and  $\gamma_j = \pi(1 - \pi)^{j-1}$  causes the LORD algorithm to produce thresholds identical to those in Eq (5).

Before proving Remark B.1, it will be helpful to introduce a recursive version of Eq (6). We define

$$\bar{W}_\lambda(t) = \alpha(1 \vee |\mathcal{R}_t|) - \sum_{i \leq t} \frac{\bar{\alpha}_i \mathbf{1}(P_i > \lambda)}{1 - \lambda}.$$

$\bar{W}_\lambda(t - 1) \times (1 - \lambda)$  can be approximately interpreted as the largest possible value for  $\alpha_t$  that still ensures  $\widehat{\text{FDP}}_\lambda(t) \leq \alpha$  (with the approximation coming from the use of  $\bar{\alpha}_i$  in the summation term, rather than  $\min\{\lambda, \bar{\alpha}_i\}$ ). Applying this notation, Eq (6) simplifies to

$$\bar{\alpha}_t = \bar{W}_\lambda(t - 1)(1 - \lambda)\pi.$$

From here, we note that  $\bar{W}_\lambda(t)$  can be written as a function of  $\bar{W}_\lambda(t-1)$ . Let

$$D_t = (1 \vee |\mathcal{R}_t|) - (1 \vee |\mathcal{R}_{t-1}|)$$

be an indicator of an increase in the number of discoveries at time  $t$ , in excess of 1 discovery. We can now write

$$\begin{aligned} \bar{W}_\lambda(t) &= \alpha \{ (1 \vee |\mathcal{R}_{t-1}|) + D_t \} \\ &\quad - \sum_{i \leq t-1} \frac{\bar{\alpha}_i \mathbf{1}(P_i > \lambda)}{1 - \lambda} - \frac{\bar{\alpha}_t \mathbf{1}(P_t > \lambda)}{1 - \lambda} \\ &= \bar{W}_\lambda(t-1) + \alpha D_t - \frac{\bar{\alpha}_t}{1 - \lambda} \times \mathbf{1}(P_t > \lambda) \\ &= \bar{W}_\lambda(t-1) + \alpha D_t - \bar{W}_\lambda(t-1) \pi \times \mathbf{1}(P_t > \lambda) \\ &= \bar{W}_\lambda(t-1) \{1 - \pi \mathbf{1}(P_t > \lambda)\} + \alpha D_t \\ &= \bar{W}_\lambda(t-1) (1 - \pi)^{\mathbf{1}(P_t > \lambda)} + \alpha D_t. \end{aligned} \tag{B.2}$$

We are now prepared to show Remark (B.1).

### Proof of Remark B.1

*Proof.* We show the result by induction. The base case of  $t = 1$  holds trivially, since

$$\tilde{\alpha}_1 = W_0 \gamma_1 = \alpha(1 - \lambda) \pi = \bar{\alpha}_1.$$

For the inductive step, we assume that  $\tilde{\alpha}_i = \bar{\alpha}_i$  for all  $i < t$ , and show that this implies  $\tilde{\alpha}_t = \bar{\alpha}_t$ .

Before continuing, we make a minor comment regarding the notation  $|\mathcal{R}_i|$ . By assumption, we know that  $\min\{\lambda, \tilde{\alpha}_i\} = \min\{\lambda, \bar{\alpha}_i\}$  for  $i < t$ . That is, we know by assumption that the hypotheses rejected in the first  $t-1$  stages of the SAFFRON algorithm are the same as those rejected in the first  $t-1$  stages according to Eq (6). For this reason, we use  $|\mathcal{R}_i|$  for  $i < t$  to refer to both the number of hypotheses rejected by SAFFRON, and, equivalently, the number of hypotheses rejected according to Eq (6).

Plugging in the definition of  $\gamma_j$  and  $W_0$ , and noting that  $r_0 < t-1$  whenever  $t > 1$ , we have

$$\begin{aligned} \tilde{\alpha}_t &= \alpha(1 - \lambda) \sum_{j=0}^{|\mathcal{R}_{t-1}|} \gamma_{1+N_{j+}(t)} \mathbf{1}(j \neq 1) \\ &= \alpha \pi (1 - \lambda) \sum_{j=0}^{|\mathcal{R}_{t-1}|} (1 - \pi)^{N_{j+}(t)} \mathbf{1}(j \neq 1). \end{aligned} \tag{B.3}$$

We can break down the  $N_{j+}(t)$  term by noting that, for any  $j < |\mathcal{R}_{t-1}|$ , we have  $r_j < r_{|\mathcal{R}_{t-1}|} \leq t-1$ , which implies that

$$N_{j+}(t) = N_{j+}(t-1) + \mathbf{1}(P_{t-1} \geq \lambda).$$

We consider two cases, depending on whether  $D_{t-1} = 0$  or  $D_{t-1} = 1$ . If  $D_{t-1} = 0$ , then either no rejections occurred at stage  $t-1$  or the first rejection occurred at stage  $t-1$ . In either case, the indices for

the summation in Eq (B.3) remain unchanged from stage  $t - 2$  to stage  $t - 1$ . Thus

$$\begin{aligned}
\tilde{\alpha}_t &= \alpha\pi(1-\lambda) \sum_{j=0}^{|\mathcal{R}_{t-2}|} (1-\pi)^{N_{j+}(t)} \mathbf{1}(j \neq 1) \\
&= \alpha\pi(1-\lambda) \sum_{j=0}^{|\mathcal{R}_{t-2}|} (1-\pi)^{N_{j+}(t-1)} (1-\pi)^{\mathbf{1}(P_{t-1} > \lambda)} \mathbf{1}(j \neq 1) \\
&= (1-\pi)^{\mathbf{1}(P_{t-1} > \lambda)} \left[ \alpha\pi(1-\lambda) \sum_{j=0}^{|\mathcal{R}_{t-2}|} (1-\pi)^{N_{j+}(t-1)} \mathbf{1}(j \neq 1) \right] \\
&= (1-\pi)^{\mathbf{1}(P_{t-1} > \lambda)} \tilde{\alpha}_{t-1} \\
&= (1-\pi)^{\mathbf{1}(P_{t-1} > \lambda)} \bar{\alpha}_{t-1} \\
&= \left\{ (1-\pi)^{\mathbf{1}(P_{t-1} > \lambda)} W_\lambda(t-2) \right\} (1-\lambda)\pi. \tag{B.4}
\end{aligned}$$

Applying Eq (B.2) with  $D_{t-1} = 0$ , we see that the term in curly braces is equal to  $W_\lambda(t-1)$ , and so  $\tilde{\alpha}_t = W_\lambda(t-1)(1-\lambda)\pi = \bar{\alpha}_t$ .

Alternatively, if  $D_{t-1} = 1$ , then  $|\mathcal{R}_{t-1}|$  must be larger than 1, and  $|\mathcal{R}_{t-1}| = 1 + |\mathcal{R}_{t-2}|$ . In this case, we also know that  $N_{|\mathcal{R}_{t-1}|+}(t) = 0$ , since the  $|\mathcal{R}_{t-1}|^{th}$  rejection happens in stage  $t-1$ , and there are no stages between  $t-1$  and  $t$ . Thus

$$\begin{aligned}
\tilde{\alpha}_t &= \alpha\pi(1-\lambda) \left( \sum_{j=0}^{|\mathcal{R}_{t-1}|} (1-\pi)^{N_{j+}(t)} \mathbf{1}(j \neq 1) \right) \\
&= \alpha\pi(1-\lambda) \left( \sum_{j=0}^{|\mathcal{R}_{t-1}|-1} (1-\pi)^{N_{j+}(t)} \mathbf{1}(j \neq 1) + (1-\pi)^{N_{|\mathcal{R}_{t-1}|+}(t)} \mathbf{1}(|\mathcal{R}_{t-1}| \neq 1) \right) \\
&= \alpha\pi(1-\lambda) \left( \sum_{j=0}^{|\mathcal{R}_{t-2}|} (1-\pi)^{N_{j+}(t)} \mathbf{1}(j \neq 1) + 1 \right) \\
&= \alpha\pi(1-\lambda) + \alpha\pi(1-\lambda) \sum_{j=0}^{|\mathcal{R}_{t-2}|} (1-\pi)^{N_{j+}(t)} \mathbf{1}(j \neq 1) \\
&= \alpha\pi(1-\lambda) + (1-\pi)^{\mathbf{1}(P_{t-1} > \lambda)} W_\lambda(t-2) (1-\lambda)\pi && \text{from Eq (B.4)} \\
&= \pi(1-\lambda) \left[ \alpha D_{t-1} + (1-\pi)^{\mathbf{1}(P_{t-1} > \lambda)} W_\lambda(t-2) \right] && \text{from } D_{t-1} = 1 \\
&= \pi(1-\lambda) W_\lambda(t-1) && \text{from Eq (B.2)} \\
&= \bar{\alpha}_t.
\end{aligned}$$

This completes the result.  $\square$

### B.3 Monotonicity of proposed algorithms

It has already been demonstrated that the LORD and SAFFRON algorithms produce thresholds that are nonincreasing in the p-values observed so far (this can immediately be seen in the algorithm definitions from Ramdas et al., 2017 and Ramdas et al., 2018). Here, we show that the additional, modified algorithms proposed in Section 4 all also produce thresholds that are nonincreasing in the p-values observed so far. In the process, we illustrate iterative formulas for the thresholds, which can be used to improve computational efficiency.

### B.3.1 LORD with dynamic spending proportions and planning ahead

Let  $\{\pi_{s_i} : i \in \mathbb{N}\}$  be a sequence of user-specified parameters, each within the interval  $[0, 1]$ , where  $s_i$  is the time by which  $\alpha_i$  must be specified. For a given p-value vector  $\mathbf{p} = (p_1, \dots, p_t)$ , we define each threshold  $\alpha_i$  as

$$\alpha_i = \left\{ \alpha (1 \vee |\mathcal{R}_{s_i}|) - \sum_{\{j: s_j < s_i\}} \alpha_j \right\} \frac{\pi_{s_i}}{n_{s_i}},$$

where  $\mathcal{R}_i = \{j \leq i : p_j \leq \alpha_j\}$ . Eqs (5) & (7) follows as special cases. Let

$$W_{0,s}(i) = \alpha (1 \vee |\mathcal{R}_{s_i}|) - \sum_{\{j: s_j < s_i\}} \alpha_j,$$

so that  $\alpha_i = W_{0,s}(s_i) \frac{\pi_{s_i}}{n_{s_i}}$ . Additionally, let  $s_{(1)} \leq \dots \leq s_{(k_{\max})}$  be the unique stages at which thresholds are defined, where  $s_{(1)} = 0$  and  $s_{(k_{\max})} = \max_{i \leq t} s_i$ , and let

$$D_{(k+1)} = (1 \vee |\mathcal{R}_{s_{(k+1)}}|) - (1 \vee |\mathcal{R}_{s_{(k)}}|)$$

be the number of new discoveries made in between stages  $s_{(k)}$  and  $s_{(k+1)}$ , in excess of 1 discovery.

Given a second p-value vector  $\mathbf{p}^* = (p_1^*, \dots, p_t^*)$  satisfying  $p_i^* \leq p_i$  for all  $i \leq t$ , let  $W_{0,s}^*(s_i)$ ,  $\alpha_i^*$ , and  $D_{(k+1)}^*$  be the analogues of  $W_{0,s}(s_i)$ ,  $\alpha_i$ , and  $D_{(k+1)}$  that would result from applying the same procedure to  $\mathbf{p}^*$  rather than  $\mathbf{p}$ . We will show the following monotonicity result.

*Remark B.2.* At every time  $s_{(k)}$  at which thresholds are defined (that is, for all  $k \in \{1, \dots, k_{\max}\}$ ), we have  $W_{0,s}(s_{(k)}) \leq W_{0,s}^*(s_{(k)})$ , and  $\alpha_i \leq \alpha_i^*$  for all  $i$  satisfying  $s_i = s_{(k)}$ .

#### Proof of Remark B.2

*Proof.* The proof is by induction. For the base case of  $k = 1$  we have  $s_{(k)} = 0$  and  $W_{0,s}(0) = \alpha = W_{0,s}^*(0)$ . Similarly, for all  $i$  satisfying  $s_i = 0$ , we have  $\alpha_i = \alpha \frac{\pi_0}{n_0} = \alpha_i^*$ .

For the induction step, assume that  $W_{0,s}(s_{(k)}) \leq W_{0,s}^*(s_{(k)})$ , and  $\alpha_i \leq \alpha_i^*$  for all  $i$  such that  $s_i \leq s_{(k)}$ . Every stage up to and including stage  $s_{(k+1)}$  must have a threshold parameter that is specified by stage  $s_{(k)}$ . That is, for any  $i \leq s_{(k+1)}$ , we must have  $s_i \leq s_{(k)}$ , which, in turn, implies that  $\alpha_i \leq \alpha_i^*$ . From here, we have

$$\begin{aligned} D_{(k+1)} &= \left( \sum_{i=s_{(k)}+1}^{s_{(k+1)}} \mathbf{1}(p_i \leq \alpha_i) \right) - \mathbf{1} \left( k = 1 \text{ or } \bigcap_{i \leq s_{(k)}} p_i > \alpha_i \right) \\ &\leq \left( \sum_{i=s_{(k)}+1}^{s_{(k+1)}} \mathbf{1}(p_i^* \leq \alpha_i^*) \right) - \mathbf{1} \left( k = 1 \text{ or } \bigcap_{i \leq s_{(k)}} p_i^* > \alpha_i^* \right) \\ &= D_{(k+1)}^*. \end{aligned} \tag{B.5}$$

Above, the second term in Line B.5 indicates the event that there were no rejections up to and including stage  $s_{(k)}$ .

Applying this, we have

$$W_{0,s}(s_{(k+1)}) = \alpha (1 \vee |\mathcal{R}_{s_{(k+1)}}|) - \left( \sum_{\{j: s_j < s_{(k)}\}} \alpha_j \right) - \left( \sum_{\{j: s_j = s_{(k)}\}} \alpha_j \right) \quad (\text{B.6})$$

$$\begin{aligned} &= \alpha (1 \vee |\mathcal{R}_{s_{(k+1)}}|) - \left( \sum_{\{j: s_j < s_{(k)}\}} \alpha_j \right) - \left( \sum_{\{j: s_j = s_{(k)}\}} W_{0,s}(s_j) \frac{\pi_{s_j}}{n_{s_j}} \right) \\ &= \alpha (1 \vee |\mathcal{R}_{s_{(k+1)}}|) - \left( \sum_{\{j: s_j < s_{(k)}\}} \alpha_j \right) - W_{0,s}(s_{(k)}) \pi_{s_{(k)}} \\ &= \alpha (1 \vee |\mathcal{R}_{s_{(k)}}|) + \alpha D_{(k+1)} - \left( \sum_{\{j: s_j < s_{(k)}\}} \alpha_j \right) - W_{0,s}(s_{(k)}) \pi_{s_{(k)}} \\ &= W_{0,s}(s_{(k)}) + \alpha D_{(k+1)} - W_{0,s}(s_{(k)}) \pi_{s_{(k)}} \\ &= W_{0,s}(s_{(k)}) (1 - \pi_{s_{(k)}}) + \alpha D_{(k+1)} \quad (\text{B.7}) \\ &\leq W_{0,s}^*(s_{(k)}) (1 - \pi_{s_{(k)}}) + \alpha D_{(k+1)}^* \\ &= W_{0,s}^*(s_{(k+1)}). \end{aligned}$$

where the last line comes from applying the steps from Lines B.6-B.7 in reverse. Finally, for all  $i$  satisfying  $s_i = s_{(k+1)}$ , we have

$$\begin{aligned} \alpha_i &= W_{0,s}(s_{(k+1)}) \frac{\pi_{s_{(k+1)}}}{n_{s_{(k+1)}}} \\ &\leq W_{0,s}^*(s_{(k+1)}) \frac{\pi_{s_{(k+1)}}}{n_{s_{(k+1)}}} \\ &= \alpha_i^*. \end{aligned}$$

This completes the result.  $\square$

### B.3.2 SAFFRON with dynamic spending proportions and planning ahead

Alternatively, suppose we define thresholds as in Eq (8), but with the option of user-specified, stage specific spending parameters  $\{\pi_{s_i} : i \in \mathbb{N}\}$ . Building on the approach in the previous subsection, let

$$W_{\lambda,s}(s_{(k)}) = \alpha (1 \vee |\mathcal{R}_{s_{(k)}}|) - \sum_{\{i: s_i < s_{(k)}\}} \frac{\alpha_i \mathbf{1}(\lambda_i < p_i \text{ or } s_{(k)} < i)}{1 - \lambda_i}, \quad (\text{B.8})$$

and let

$$\alpha_i = \min \left\{ W_{\lambda,s}(s_i) (1 - \lambda_i) \frac{\pi_{s_i}}{n_{s_i}}, \lambda_i \right\}. \quad (\text{B.9})$$

Eq (8) is the special case of Eqs (B.8)-(B.9) when all parameters  $\pi_i$  are equal, and Eq (6) is the special case where, additionally,  $\lambda_i = \lambda$  and  $s_i = i - 1$  for all  $i \in \mathbb{N}$ .

Let  $\mathbf{p}^* = (p_1^*, \dots, p_t^*)$  and  $D_{(k+1)}^*$  be defined as in the previous section, and let  $W_{\lambda,s}^*(s_i)$ ,  $\alpha_i^*$ , and  $D_{(k+1)}^*$  be the analogues of  $W_{\lambda,s}(s_i)$ ,  $\alpha_i$ , and  $D_{(k+1)}$  that would result from applying the same procedure (Eqs (B.8)-(B.9)) to  $\mathbf{p}^*$  rather than  $\mathbf{p}$ . We will show the following monotonicity result.

*Remark B.3. At every time  $s_{(k)}$  at which thresholds are defined, we have  $W_{\lambda,s}(s_{(k)}) \leq W_{\lambda,s}^*(s_{(k)})$ , and  $\alpha_i \leq \alpha_i^*$  for all  $i$  satisfying  $s_i = s_{(k)}$ .*

### Proof of Remark B.3

*Proof.* Again, the proof is by induction. For the base case of  $k = 1$  we have  $s_{(k)} = 0$  and  $W_{\lambda,s}(0) = \alpha = W_{\lambda,s}^*(0)$ . Similarly, for all  $i$  satisfying  $s_i = 0$ , we have  $\alpha_i = \min \left\{ \alpha (1 - \lambda_i)^{\frac{\pi_0}{n_0}}, \lambda_i \right\} = \alpha_i^*$ .

For the induction step, assume that  $W_{\lambda,s}(s_{(k)}) \leq W_{\lambda,s}^*(s_{(k)})$ , and  $\alpha_i \leq \alpha_i^*$  for all  $i$  such that  $s_i \leq s_{(k)}$ . By the same logic as in Section B.3.1, we know that  $D_{(k+1)} \leq D_{(k+1)}^*$ , and that  $\alpha_i \leq \alpha_i^*$  for all  $i \leq s_{(k+1)}$ .

We begin by describing  $W_{\lambda,s}(s_{(k+1)})$  as a function of  $W_{\lambda,s}(s_{(k)})$ . We see that

$$W_{\lambda,s}(s_{(k+1)}) = \alpha D_{(k+1)} + \alpha (1 \vee |\mathcal{R}_{s_{(k)}}|) - \sum_{\{i: s_i \leq s_{(k)}\}} \frac{\alpha_i \mathbf{1}(\lambda_i < p_i \text{ or } s_{(k+1)} < i)}{1 - \lambda_i} \quad (\text{B.10})$$

For each of the summation terms in Line B.10, we note that

$$\begin{aligned} -\mathbf{1}(\lambda_i < p_i \text{ or } s_{(k+1)} < i) &= \mathbf{1}(\lambda_i < p_i \text{ or } s_{(k)} < i) - \mathbf{1}(\lambda_i < p_i \text{ or } s_{(k+1)} < i) \\ &\quad - \mathbf{1}(\lambda_i < p_i \text{ or } s_{(k)} < i) \\ &= \mathbf{1}(\lambda_i \geq p_i \text{ and } s_{(k)} < i \leq s_{(k+1)}) \\ &\quad - \mathbf{1}(\lambda_i < p_i \text{ or } s_{(k)} < i). \end{aligned}$$

Plugging this in, we have

$$W_{\lambda,s}(s_{(k+1)}) = \alpha D_{(k+1)} + \sum_{\{i: s_i \leq s_{(k)}\}} \frac{\alpha_i \mathbf{1}(\lambda_i \geq p_i \text{ and } s_{(k)} < i \leq s_{(k+1)})}{1 - \lambda_i} \quad (\text{B.11})$$

$$+ \alpha (1 \vee |\mathcal{R}_{s_{(k)}}|) - \sum_{\{i: s_i \leq s_{(k)}\}} \frac{\alpha_i \mathbf{1}(\lambda_i < p_i \text{ or } s_{(k)} < i)}{1 - \lambda_i} \quad (\text{B.12})$$

$$= \alpha D_{(k+1)} + \sum_{i=s_{(k)}+1}^{s_{(k+1)}} \frac{\alpha_i \mathbf{1}(\lambda_i \geq p_i)}{1 - \lambda_i} \quad (\text{B.13})$$

$$W_{\lambda,s}(s_{(k)}) - \sum_{\{i: s_i = s_{(k)}\}} \frac{\alpha_i \mathbf{1}(\lambda_i < p_i \text{ or } s_{(k)} < i)}{1 - \lambda_i}. \quad (\text{B.14})$$

To transform Line (B.11) to Line B.13, we use the fact that  $i \leq s_{(k+1)}$  implies that  $s_i \leq s_{(k)}$ , making the condition in the summation index redundant. To transform Line (B.12) to Line (B.14), we plug in the definition of  $W_{\lambda,s}(s_{(k)})$ . Intuitively, Lines (B.11)-(B.14) say that the difference in wealth between stages  $s_{(k+1)}$  and  $s_{(k)}$  is equal to  $\alpha$  times the number of new rejections (in excess of 1, i.e.,  $\alpha D_{(k+1)}$ ), minus a conservative estimate of the alpha cost for thresholds specified at stage  $s_{(k)}$  (the summation in Line (B.14)), plus a correction for any such alpha cost estimate that is newly shown to be *overly* conservative (the summation in Line (B.13)).

To study Line (B.14) in more detail, we will use  $\mathcal{I}_{(k)} = \{i : s_i = s_{(k)} \text{ and } (\lambda_i < p_i \text{ or } s_{(k)} < i)\}$  to refer to

the indices of the nonzero terms in the summation. Line (B.14) is equal to

$$\begin{aligned}
W_{\lambda,s}(s_{(k)}) &= \sum_{\{i:s_i=s_{(k)}\}} \frac{\alpha_i \mathbf{1}(\lambda_i < p_i \text{ or } s_{(k)} < i)}{1 - \lambda_i} \\
&= W_{\lambda,s}(s_{(k)}) - \sum_{i \in \mathcal{I}_{(k)}} \frac{\alpha_i}{1 - \lambda_i} \\
&= W_{\lambda,s}(s_{(k)}) - \sum_{i \in \mathcal{I}_{(k)}} \min \left\{ \frac{W_{\lambda,s}(s_{(k)}) \pi_{s_{(k)}}}{n_{s_{(k)}}}, \frac{\lambda_i}{1 - \lambda_i} \right\} \\
&= W_{\lambda,s}(s_{(k)}) + \sum_{i \in \mathcal{I}_{(k)}} \max \left\{ \frac{-W_{\lambda,s}(s_{(k)}) \pi_{s_{(k)}}}{n_{s_{(k)}}}, \frac{-\lambda_i}{1 - \lambda_i} \right\} \\
&= \sum_{i \in \mathcal{I}_{(k)}} \frac{W_{\lambda,s}(s_{(k)})}{|\mathcal{I}_{(k)}|} + \max \left\{ \frac{-W_{\lambda,s}(s_i) \pi_{s_{(k)}}}{n_{s_{(k)}}}, \frac{-\lambda_i}{1 - \lambda_i} \right\} \\
&= \sum_{i \in \mathcal{I}_{(k)}} \max \left\{ \frac{W_{\lambda,s}(s_{(k)})}{|\mathcal{I}_{(k)}|} - \frac{W_{\lambda,s}(s_{(k)}) \pi_{s_{(k)}}}{n_{s_{(k)}}}, \frac{W_{\lambda,s}(s_{(k)})}{|\mathcal{I}_{(k)}|} - \frac{\lambda_i}{1 - \lambda_i} \right\} \\
&\leq \sum_{i \in \mathcal{I}_{(k)}} \max \left\{ \frac{W_{\lambda,s}^*(s_{(k)})}{|\mathcal{I}_{(k)}|} - \frac{W_{\lambda,s}^*(s_i) \pi_{s_i}}{n_{s_i}}, \frac{W_{\lambda,s}^*(s_{(k)})}{|\mathcal{I}_{(k)}|} - \frac{\lambda_i}{1 - \lambda_i} \right\} \tag{B.15}
\end{aligned}$$

$$= W_{\lambda,s}^*(s_{(k)}) - \sum_{i \in \mathcal{I}_{(k)}} \frac{\alpha_i^*}{1 - \lambda_i} \tag{B.16}$$

Above, Line B.15 comes from the fact that  $1/n_{s_i} \leq 1/|\mathcal{I}_{(k)}|$ .

Combining Eqs B.14 & B.16 with the fact that  $D_{(k+1)} \leq D_{(k+1)}^*$ , and  $\alpha_i \leq \alpha_i^*$  for all  $i \leq s_{(k+1)}$ , we see that

$$\begin{aligned}
W_{\lambda,s}(s_{(k+1)}) &= \alpha D_{(k+1)} + \sum_{i=s_{(k)}+1}^{s_{(k+1)}} \frac{\alpha_i \mathbf{1}(\lambda_i \geq p_i)}{1 - \lambda_i} + W_{\lambda,s}(s_{(k)}) - \sum_{i \in \mathcal{I}_{(k)}} \frac{\alpha_i}{1 - \lambda_i} \\
&\leq \alpha D_{(k+1)}^* + \sum_{i=s_{(k)}+1}^{s_{(k+1)}} \frac{\alpha_i^* \mathbf{1}(\lambda_i \geq p_i)}{1 - \lambda_i} + W_{\lambda,s}^*(s_{(k)}) - \sum_{i \in \mathcal{I}_{(k)}} \frac{\alpha_i^*}{1 - \lambda_i} \\
&= W_{\lambda,s}^*(s_{(k+1)}).
\end{aligned}$$

Finally, for all  $i$  such that  $s_i = s_{(k+1)}$ , we have

$$\begin{aligned}
\alpha_i &= \min \left\{ W_{\lambda,s}(s_{(k+1)}) (1 - \lambda_i) \frac{\pi_{s_i}}{n_{s_i}}, \lambda_i \right\} \\
&\leq \min \left\{ W_{\lambda,s}^*(s_{(k+1)}) (1 - \lambda_i) \frac{\pi_{s_i}}{n_{s_i}}, \lambda_i \right\} \\
&= \alpha_i^*.
\end{aligned}$$

This completes the proof. □

## References

Blanchard, G. and Roquain, E. (2008). Two simple sufficient conditions for FDR control. *EJSS*, 2(none):963–992.

- Ramdas, A., Yang, F., Wainwright, M. J., and Jordan, M. I. (2017). Online control of the false discovery rate with decaying memory. In Guyon, I., Luxburg, U. V., Bengio, S., Wallach, H., Fergus, R., Vishwanathan, S., and Garnett, R., editors, *Advances in Neural Information Processing Systems*, volume 30. Curran Associates, Inc.
- Ramdas, A., Zrnic, T., Wainwright, M., and Jordan, M. (2018). SAFFRON: an adaptive algorithm for online control of the false discovery rate. In Dy, J. and Krause, A., editors, *Proceedings of the 35th International Conference on Machine Learning*, volume 80 of *Proceedings of Machine Learning Research*, pages 4286–4294. PMLR.
- Wolfstetter, E., Dulleck, U., Inderst, R., Kuhbier, P., and Lands-Berger, M. (1993). *Stochastic dominance: theory and applications*. Citeseer.
